# Supplementary material for: Separability in B\"uchi Vass and Singly Non-Linear Systems of Inequalities
Source: arXiv:2406.01008 source file (2024-06-03)
Supplement: Supplementary file 1 [file appendix.tex]

\section{Proofs}
\subsection{The Algorithm}
\begin{theorem}\label{Theorem:MainResult}
    $\omega$-$\mathsf{VASS}$-$\mathsf{REGSEP}$ is $\EXPSPACE$ complete. 
\end{theorem}

We prove the upper bound of Theorem~\ref{Theorem:MainResult} by giving an algorithm.
Our algorithm consists of two checks for each configuration $(q, c)\in\states\times\nat^{d+n}$.
First, we check whether $\replacein{c}{\counters}{k}$ is coverable from $(q_0, \zerovec)$ in $\avass\times\dyckvass{n}$ for all $k\in\nat$.
Then, we check whether $(\finalstate, c')\in\finalstates\times\natomega^{d+n}$ is coverable from $(q, \replacein{c}{\counters}{\omega})$, where $((\finalstate, c'), \counters, \alpha, \beta, \gamma)$ is an inseparability bloom for some $\alpha, \beta,\gamma\in\loopsof{\avass\times\dyckvass{n}}$.
By Lemma~\ref{Lemma:ShortWitness}, the latter check only needs to explore loops $\alpha$, $\beta$, $\gamma$ of size at most $f(\counters)\leq \sizeof{\avass}^{2^{\bigoof{\sizeof{\counters}^k}}}$.

\begin{proof}
    Our algorithm is a non-deterministic, space bounded algorithm.
    It guesses a set of counters $\counters\subseteq\set{0, \ldots, d+n}$, and a configuration $(q,c)\in\finalstates\times\nat^{d+n}$ with $c[i]\leq \largesteffof{\avass}\cdot\sizeof{\avass}^{2^{\bigoof{\sizeof{\counters}^k}}}$ for all $i\in\set{0, \ldots, d+n}$.
    Then the algorithm performs two checks.
    If both of these checks succeed, it returns true, and if not, it moves on to the next iteration.
    It first makes a call to check whether $\iscoverable{\avass}{\replacein{c}{\counters}{\omega}}$ holds.
    This refers to the coverability of $c'_{k}=\replacein{c'}{J}{k}$ is coverable in $\avass$, where $J=\setcond{i}{c'[i]=\omega}$.
    This can be done in $(\sizeof{\avass}\cdot \sizeof{\avass}^{2^{\bigoof{\sizeof{\counters}^k}}})^{2^\bigoof{\sizeof{\counters}^b}}$ space \cite{citationneeded}, for some constant $b$ independent of $\avass$.
    If this check succeeds, the algorithm guesses some sequence of edges $\alpha$, $\beta$, $\gamma$ of size at most $\sizeof{\avass}^{2^{\bigoof{\sizeof{\counters}^k}}}$ and keeps in memory the reached configuration $(q', c')\in\states\times\natomega^{d+n}$ along with the effects $\allbalanceof{\alpha}$, $\allbalanceof{\beta}$, and $\allbalanceof{\gamma}$.
    The algorithm rejects if $(q', c')\geq (\finalstate, c)$ does not hold for any of $\alpha$, $\beta$, $\gamma$.
    Finally the algorithm verifies whether $((\finalstate, c), \counters, \alpha, \beta, \gamma)$ is a concrete inseparability bloom, by checking the last three conditions.
    That $\alpha$, $\beta$, and $\gamma$ cover $(\finalstate, c)$ from $(\finalstate, c)$ has already been insured.
    The last three conditions can be checked by basic arithmatic on vectors $\allbalanceof{\alpha}$, $\allbalanceof{\beta}$, and $\allbalanceof{\gamma}$.
    This algorithm is in $\mathsf{NEXPSPACE}\subseteq\mathsf{EXPSPACE}$.
    
    Now we argue for correctness.
    We show that there is a concrete inseparability flower in $\avass$ if and only if the algorithm returns true.
    The backward direction is clear.
    The algorithm searches for concrete inseparability flowers of bounded size, so a witness is guaranteed if the algorithm returns true.
    For the other direction, let $\avass$ contain a concrete inseparability flower $((\finalstate,c), \counters, \alpha_{0}, \beta_{0}, \gamma_{0})$.
    Let $c_{\omega}=\replacein{c}{\counters}{\omega}$.
    There is a trivial run from $(\finalstate, c_{\omega})$ that covers $(\finalstate,c_{\omega})$, and $((\finalstate, c), \counters, \alpha_{0}, \beta_{0}, \gamma_{0})$ is a concrete inseparability bloom.
    Then, by Lemma~\ref{Lemma:ShortWitness}, there is a concrete inseparability bloom $((\finalstate', c'), \counters, \alpha, \beta, \gamma)$ with $\alpha$, $\beta$, $\gamma$ having size at most $f(\counters)\leq\sizeof{\avass}^{2^{\bigoof{n^k}}}$, and $(\finalstate', c'_{\omega})$ being coverable from $(\finalstate, c_{\omega})$, where $c_{\omega}'=\replacein{c}{\counters}{\omega}$.
    Let $h_{\omega}\in\nat^{d+n}_{\omega}$ with $h_{\omega}[i]=0$ if $c_{\omega}[i]=\omega$, $h_{\omega}[i]=\min(\largesteffof{\avass}\cdot\sizeof{\avass}^{2^{\bigoof{n^k}}}, c_{\omega}'[i])$ else, for all $i\in\set{0, \ldots, d+n-1}$.
    Because any prefix of $\alpha$, $\beta$, and $\gamma$ can decrease counters by at most $\largesteffof{\avass}\cdot\sizeof{\avass}^{2^{\bigoof{n^k}}}$ tokens, we know that $((\finalstate', h_{\omega}), \counters, \alpha, \beta, \gamma)$ is an inseparability bloom.
    Furtermore, we know $(\finalstate, \replacein{c}{\counters}{k})$ is coverable from $(q_0, \zerovec)$ for all $k\in\nat$, and $(\finalstate', c_{\omega}')$ is coverable from $(\finalstate, c_{\omega})$.
    Then, $(\finalstate', \replacein{c_{\omega}'}{\counters}{k})$ is coverable from $(q_0, \zerovec)$ for all $k\in\nat$.
    Because we have $\replacein{h_\omega}{\counters}{k}\leq\replacein{c_\omega'}{\counters}{k}$ for all $k\in\nat$, we know that $(\finalstate', \replacein{h_{\omega}}{\counters}{k})$ is coverable from $(q_0, \zerovec)$ for all $k\in\nat$.
    Then $((\finalstate', h_{\omega}), \counters, \alpha, \beta, \gamma)$ is an inseparability flower in $\avass$.
    Since the counters of $h_{\omega}$ are bounded from above by $\largesteffof{\avass}\cdot\sizeof{\avass}^{2^{\bigoof{n^k}}}$, and $\alpha$, $\beta$, $\gamma$ have size at most $\largesteffof{\avass}\cdot\sizeof{\avass}^{2^{\bigoof{n^k}}}$, our algorithm would find this inseparability flower.
    This concludes the proof.
\end{proof}

\subsection{Short Witnesses}
\begin{proof}
    We let $l=2^{\sizeof{\avass}}$ and show that 
    $$f(h+1)\leq (l^{2}\sizeof{\states}\cdot f(h))^{\bigoof{\sizeof{\combinedcounters}^{6}}}\qquad f(0)\leq (l^{2}\sizeof{\states})^{\bigoof{\sizeof{\combinedcounters}^{6}}}.$$

    Base Case, $h=0$: 
    This is already clear from Lemma~\ref{Lemma:RBoundedWitnesses}.
    Boundedness is a trivial condition for $\counters=\emptyset$, so if there is a partial witness $W=(\apath, \emptyset, \alpha, \beta, \gamma)$ from $(q, c)$, it is already $1$-bounded.
    So there is a witness $W'$ from $(q, c)$ with $\sizeof{W'}\leq (l\sizeof{\states})^{\bigoof{\sizeof{\combinedcounters}^{6}}}$.

    Inductive Case, $\sizeof{\counters}=h+1$:
    Let $(q, c)$ be a configuration, and let $W=(\apath, \counters, \alpha, \beta, \gamma)$ be a $\countersp$-repeating partial witness from $(q, c)$ with $\sizeof{\counters}=h+1$.
    This case is broken down into two subcases.
    First, let $W$ be $l\cdot f(h)$-bounded.
    Then, we invoke Lemma~\ref{Lemma:RBoundedWitnesses} to show that there is a $W'$ from $(q, c)$ with $\sizeof{W'}\leq (l \cdot \sizeof{\states} \cdot l \cdot f(h))^{\bigoof{\sizeof{\combinedcounters}^{6}}}=(l^{2}\sizeof{\states}\cdot f(h))^{\bigoof{\sizeof{\combinedcounters}^{6}}}$.

    Second, let $W$ not be $l\cdot f(h)$-bounded.
    Let $\combinedcounters=\counters\uplus\omegacounters$, let $\apath$ reach $(\finalstate, \replacein{c_{f}}{\omegacounters}{\omega})$ from $(q, \replacein{c}{\omegacounters}{\omega})$, and let $((\finalstate, c_{f}), \counters, \alpha, \beta, \gamma)$ be an inseparability bloom.
    Then, let $\apath'$ be the shortest path that is a prefix of $\apath.\alpha$, $\apath.\beta$ or $\apath.\gamma$ and that reaches $(q', \replacein{c'}{\omegacounters}{\omega})$ from $(q, \replacein{c}{\omegacounters}{\omega})$, where $c'[i]>l\cdot f(h)$ for some $i\in\counters$.
    Let $\apath.\xi=\apath'.\xi'$ for some $\xi\in\set{\alpha, \beta, \gamma}$ and suffix $\xi'$ of $\apath.\xi$.

    We make three observations.
    First, there is a $\apath''$ with $\sizeof{\apath''}\leq (l \cdot \sizeof{\states}\cdot f(h))^{\sizeof{\combinedcounters}}$ that reaches $(q', \replacein{c'}{\omegacounters}{\omega})$ 
    from $(q, \replacein{c}{\omegacounters}{\omega})$.
    This is because there are at most $(l \cdot \sizeof{\states}\cdot f(h))^{\sizeof{\combinedcounters}}$ configurations with $\counters$ counters bounded by $l\cdot f(h)$ and $\omegacounters$ counters equal to $\omega$.
    Second, the loops $\alpha$, $\beta$, and $\gamma$ cover $(\finalstate, \replacein{c_{f}}{\omegacounters}{\omega})$ from $(\finalstate, \replacein{c_{f}}{\omegacounters}{\omega})$.
    Then, $\apath\cdot\xi$ covers $(\finalstate, \replacein{c_{f}}{\omegacounters}{\omega})$ from $(q, \replacein{c}{\omegacounters}{\omega})$.
    As $\apath=\apath'.\xi'$, we know that $\xi'$ reaches $(\finalstate, \replacein{c_{f}}{\omegacounters}{\omega})$ from $(q', \replacein{c'}{\omegacounters}{\omega})$,.
    Then, $(\xi', \counters, \alpha, \beta, \gamma)$ is a partial witness from $(q', c')$ that is $\countersp$-repeating.
    Finally, we observe that there is a partial witness $(\xi', \counters\setminus\set{i}, \alpha, \beta, \gamma)$ from $(q', c')$ that is $\countersp\cup\set{i}$-repeating from $(q', c')$.
    With this, we can invoke the induction hypothesis, and get a partial witness $W^{*}=(\apath^{*}, \counters\setminus\set{i}, \alpha^{*}, \beta^{*}, \gamma^{*})$ from $(q', c')$ with $\sizeof{W^{*}}\leq f(h)$ that is $\countersp\cup\set{i}$-repeating.
    We argue that $(\apath^{*}, \counters, \alpha^{*}, \beta^{*}, \gamma^{*})$ is a $\countersp$-repeating partial witness from $(q', c')$.
    We only need to verify the positivity conditions on $\counters$ counters and that the loops $\alpha$, $\beta$, $\gamma$ have a positive effect on these counters.
    The latter is guaranteed by $W^{*}$ being $\countersp\cup\set{i}$-repeating.
    We also know that the former condition holds for all counters in $\counters\setminus\set{i}$. 
    For counter $i\in\counters$, we observe that taking any prefix of $\apath^{*}.\alpha^{*}$, $\apath^{*}.\beta^{*}$, or $\apath^{*}.\gamma^{*}$ 
    can take away at most $l\cdot\sizeof{W^{*}}\leq l\cdot f(h)$ tokens from a counter.
    Since $c'[i]>l\cdot f(h)$ we know that counter $i$ always has a positive evaluation along $\apath^{*}.\alpha^{*}$, $\apath^{*}.\beta^{*}$, or $\apath^{*}.\gamma^{*}$ from $(q', \replacein{c'}{\omegacounters}{\omega})$.
    Because taking $\apath''$ from $(q, \replacein{c}{\omegacounters}{\omega})$ leads to $(q', \replacein{c'}{\omegacounters}{\omega})$, we know that $W^{**}=(\apath''.\apath^{*}, \counters, \alpha, \beta, \gamma)$ is a partial witness from $(q, c)$.
    We have $\sizeof{W^{**}}\leq (l\cdot f(h))^{\sizeof{\combinedcounters}}+f(h)$.
    
    Combining the observations of the two subcases, we get 
    \begin{align*}
        f(h+1)&\leq \max((l\cdot f(h))^{\sizeof{\combinedcounters}}+f(h), (l^{2}  \sizeof{\states}\cdot f(h))^{\sizeof{\combinedcounters}})\\
        &\leq \max(2\cdot(l\cdot f(h))^{\sizeof{\combinedcounters}},  (l^{2} \sizeof{\states}\cdot f(h))^{\sizeof{\combinedcounters}})\\
        &\leq (l^{2} \sizeof{\states}\cdot f(h))^{\sizeof{\combinedcounters}}.
    \end{align*}
\end{proof}
\newpage
\newpage
